# Supplementary material for: DAFA: Distance-Aware Fair Adversarial Training
Source: arXiv:2401.12532 source file (2024-01-23)
Supplement: Supplementary file 1 [file fig_appendix_ablations_2.tex]

\begin{figure}[t]
% \subfloat[\label{fig:introduction_tsne_clsall}]{
% \includegraphics[width=0.32\linewidth]{_fig/_fig_introduction_tsne_cls_from_trades110.pdf}}
%\hfill
\subfloat[\label{fig:appendix_cw_accuracy}]{
\includegraphics[width=0.42\linewidth]{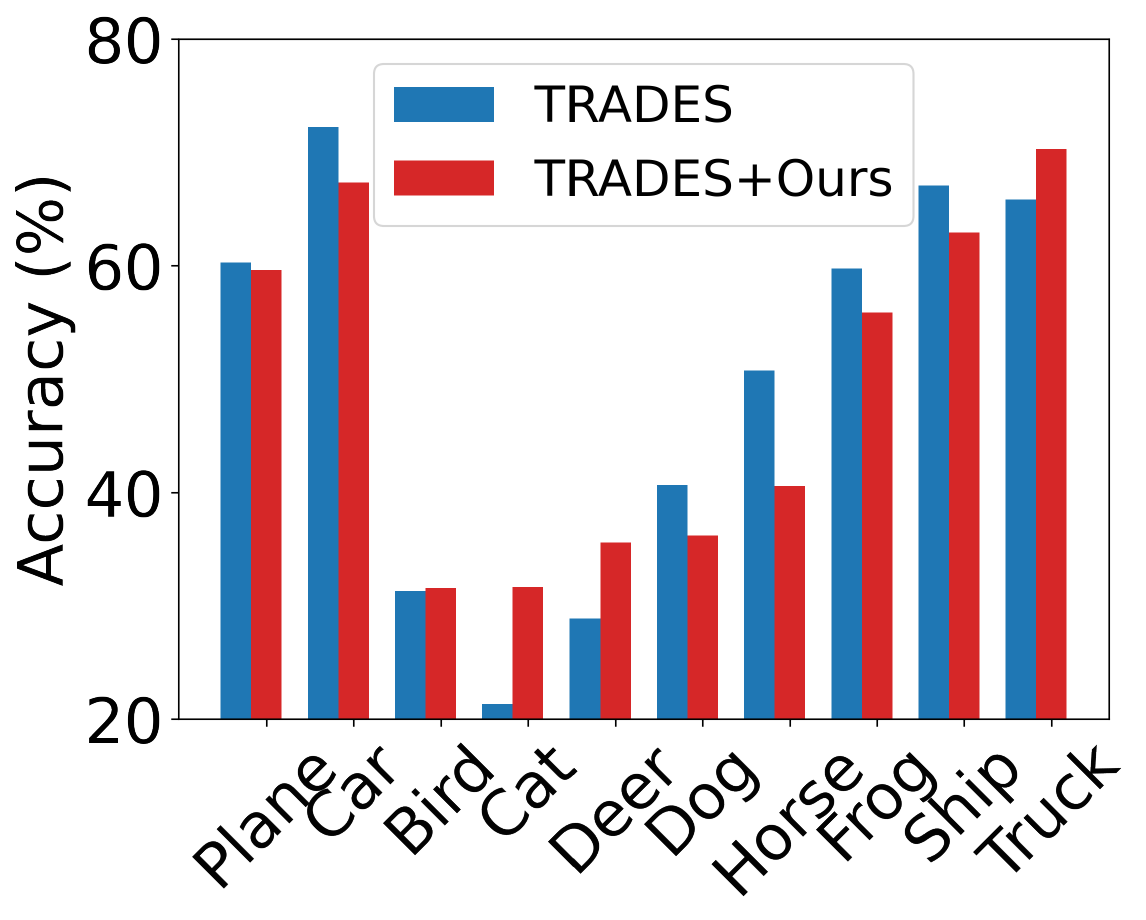}
}
\hfill
\subfloat[\label{fig:appendix_eps6_6_bird_cat_accuracy_pgd}]{
\includegraphics[width=0.42\linewidth]{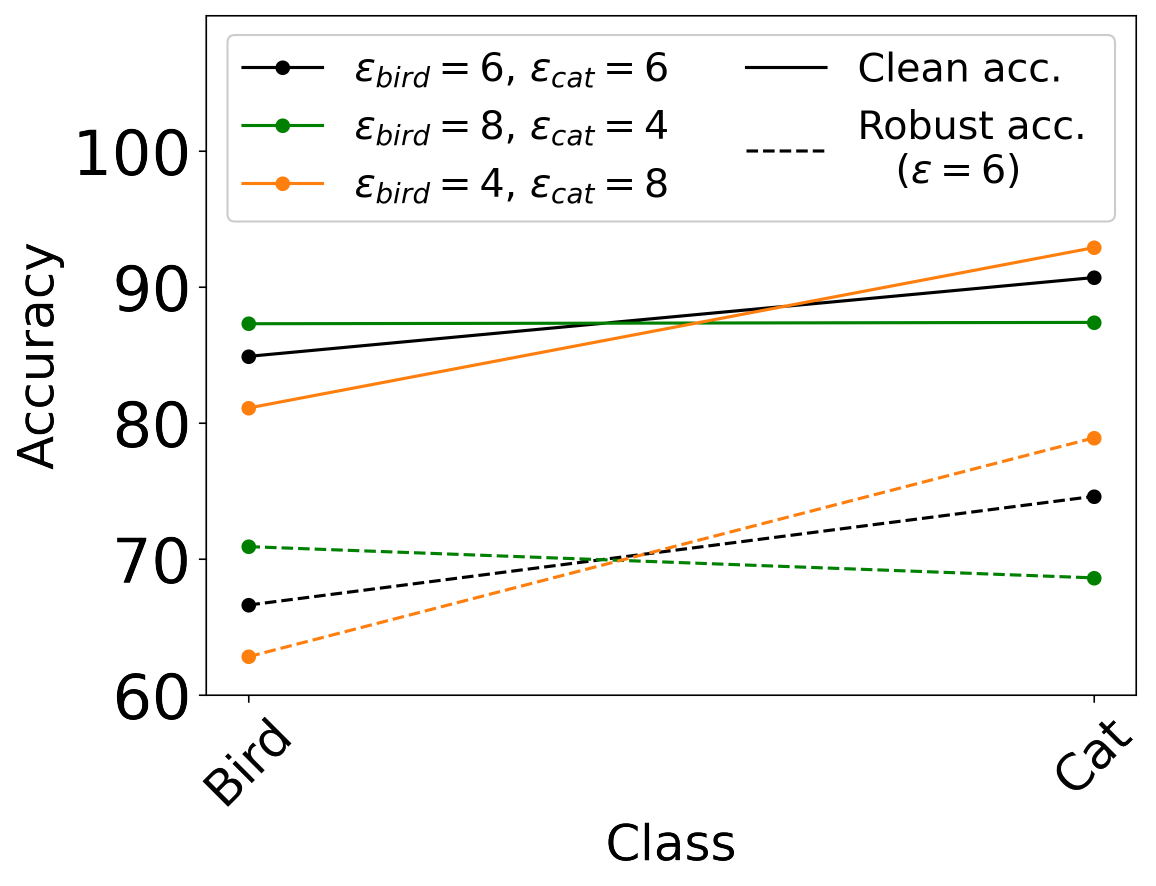}}

\caption{(a) depicts the class-wise robust accuracy for the TRADES model and its counterpart trained with DAFA. (b) Presents the results from an experiment on the PGD \citep{attack_pgd} model, mirroring the conditions of Fig. \ref{fig:method_eps6_6_bird_cat_accuracy}.}

% \caption{(a)는 TRADES 모델과 이 모델에 DAFA를 적용하여 학습된 모델의 class-wise robust accuracy를 나타낸다. (b)는 PGD \citep{attack_pgd} 모델에 Fig. \ref{fig:method_eps6_6_bird_cat_accuracy}과 동일한 실험을 한 결과를 나타낸다.}

% \vskip -2mm
%\end{center}
\label{fig:appendix_2}
\end{figure}
