# Supplementary material for: DAFA: Distance-Aware Fair Adversarial Training
Source: arXiv:2401.12532 source file (2024-01-23)
Supplement: Supplementary file 2 [file tab_appendix_analysis_corrolary.tex]

\begin{wraptable}[8]{r}{0.4\linewidth}
\centering
% \footnotesize
% \addtolength{\tabcolsep}{-0pt}
\vskip -3mm
\caption{Performance comparison of cat and dog in unconventional contexts. }
% \vskip -2mm
\begin{tabular}{c|ccc}
    \toprule     
     Model & Dog & Cat & Diff. \\
     
     % & \multicolumn{1}{c}{$\rho_{rob}$} \\
   
    \midrule[.05em]
     Std. model & 84.21 & 78.06 & 6.15 \\
     Rob. model & 47.50 & 46.10 & 1.40 \\    
    \midrule[.1em]
\end{tabular}
\label{tab:appendix_corollary}
\end{wraptable}
